# Supplementary material for: Thermoelectric properties of high-entropy rare-earth cobaltates
Source: arXiv:2206.11106 source file (2022-06-22)
Supplement: Supplementary file 1 [file Supporting_Information_Final.pdf]

## Supporting Information

### Thermoelectric Properties of high-entropy rare-earth cobaltates

Ashutosh Kumar, Diana Dragoë, David Bérardan, Nita Dragoë\*

ICMMO (UMR CNRS 8182), Université Paris-Saclay, F-91405 Orsay, France

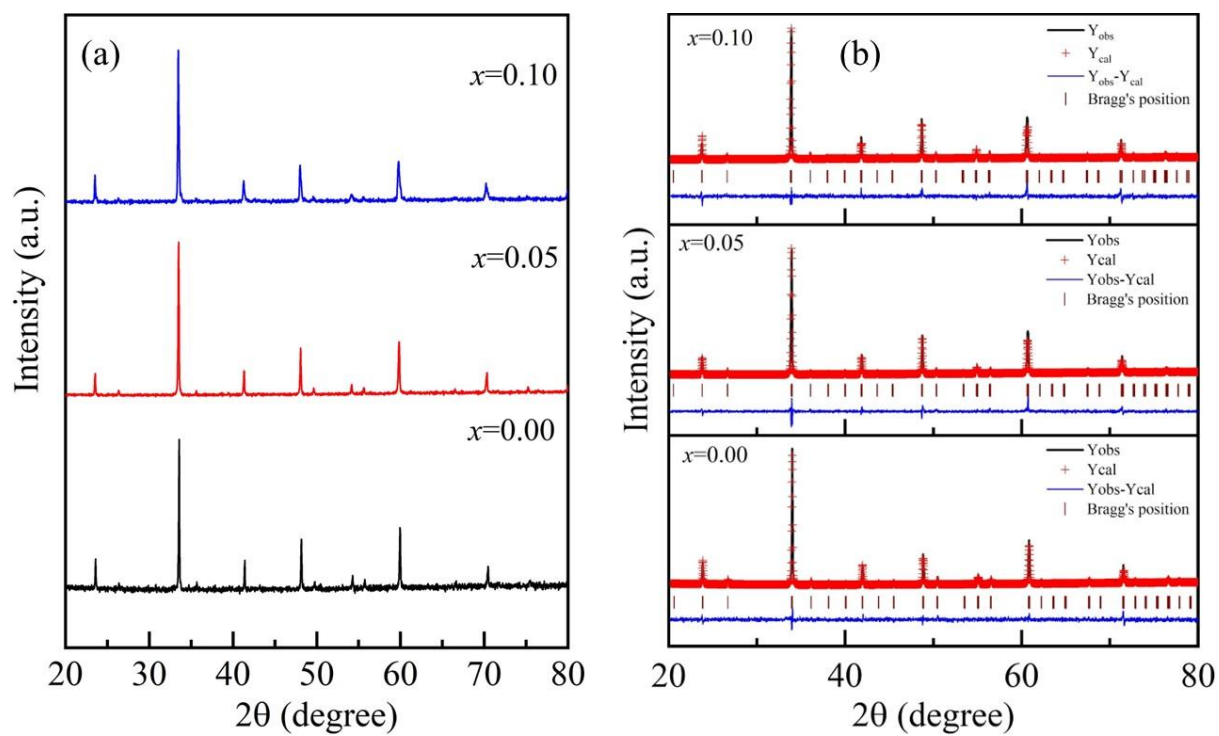

Fig.S1: (a) XRD pattern, (b) Rietveld refinement pattern of  $(\text{LaNdPrSmEu})_{1-x}\text{Sr}_x\text{CoO}_3$ .

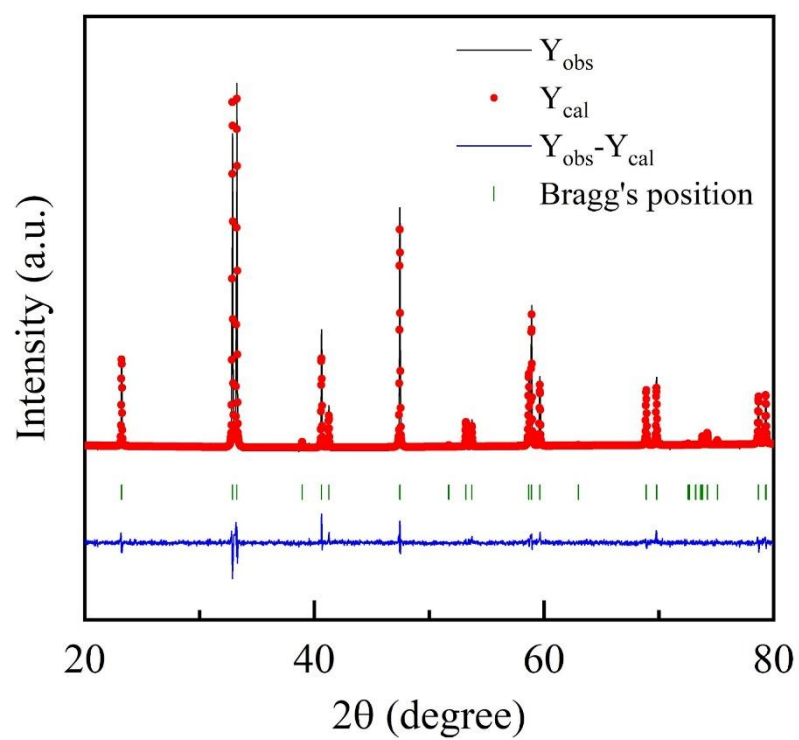

Fig.S2: Rietveld refinement pattern of  $\text{La}_{0.95}\text{Sr}_{0.05}\text{CoO}_3$ .

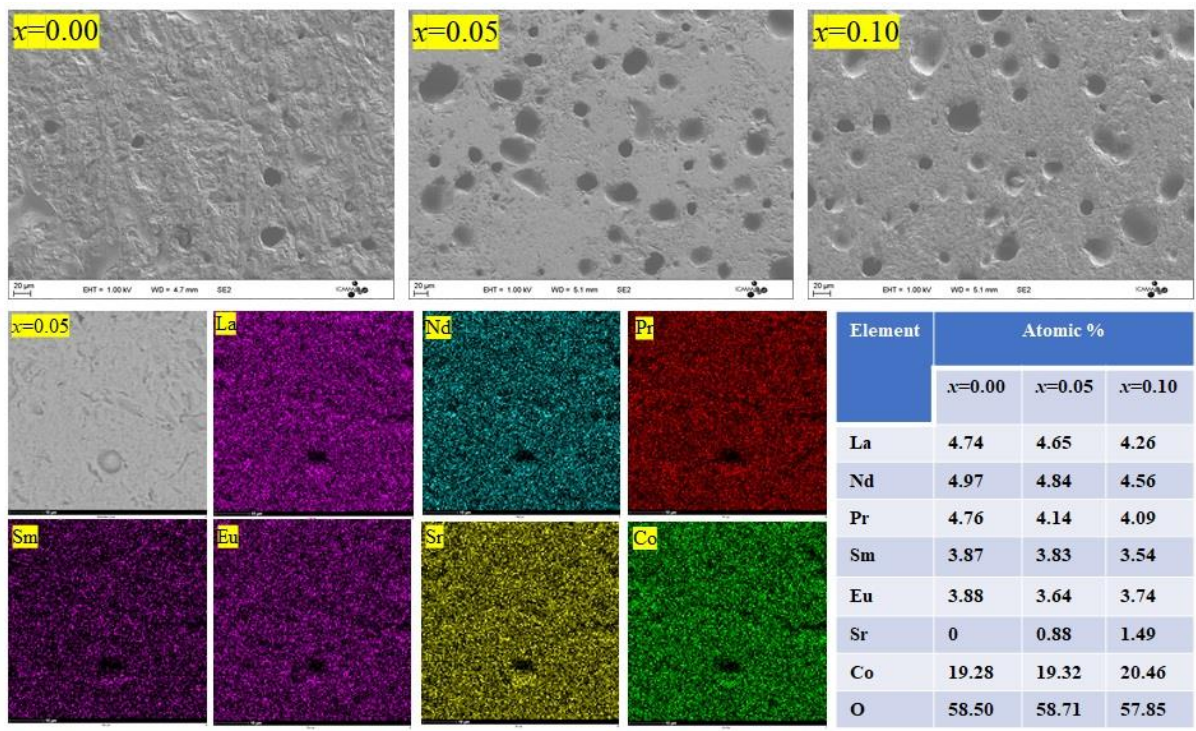

Fig.S3: Scanning electron microscope (SEM) images for  $(\text{LaNdPrSmEu})_{1-x}\text{Sr}_x\text{CoO}_3$ . The elemental mapping was done for all the samples, ( $x=0.05$  is shown). The energy dispersive x-ray analysis was performed to estimate the atomic percentage for each sample.

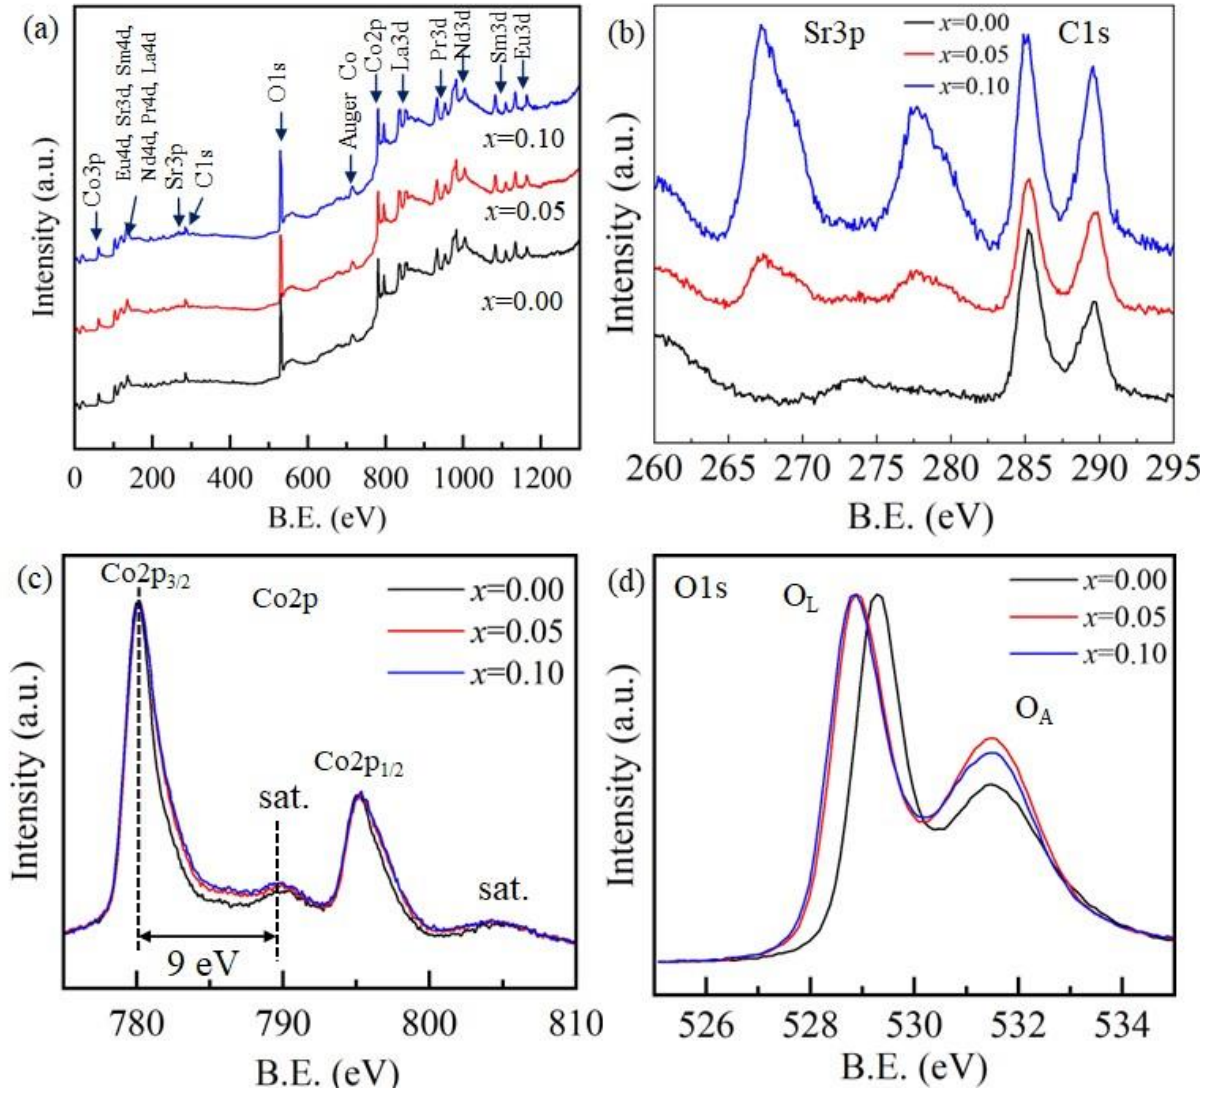

Fig.S4: (a) Full-scan X-ray photoelectron spectroscopy (XPS) measurement for  $(\text{LaNdPrSmEu})_{1-x}\text{Sr}_x\text{CoO}_3$ . Core-level spectrum for (b) Sr3d, (c) Co2p and (d) O1s for  $(\text{LaNdPrSmEu})_{1-x}\text{Sr}_x\text{CoO}_3$ .

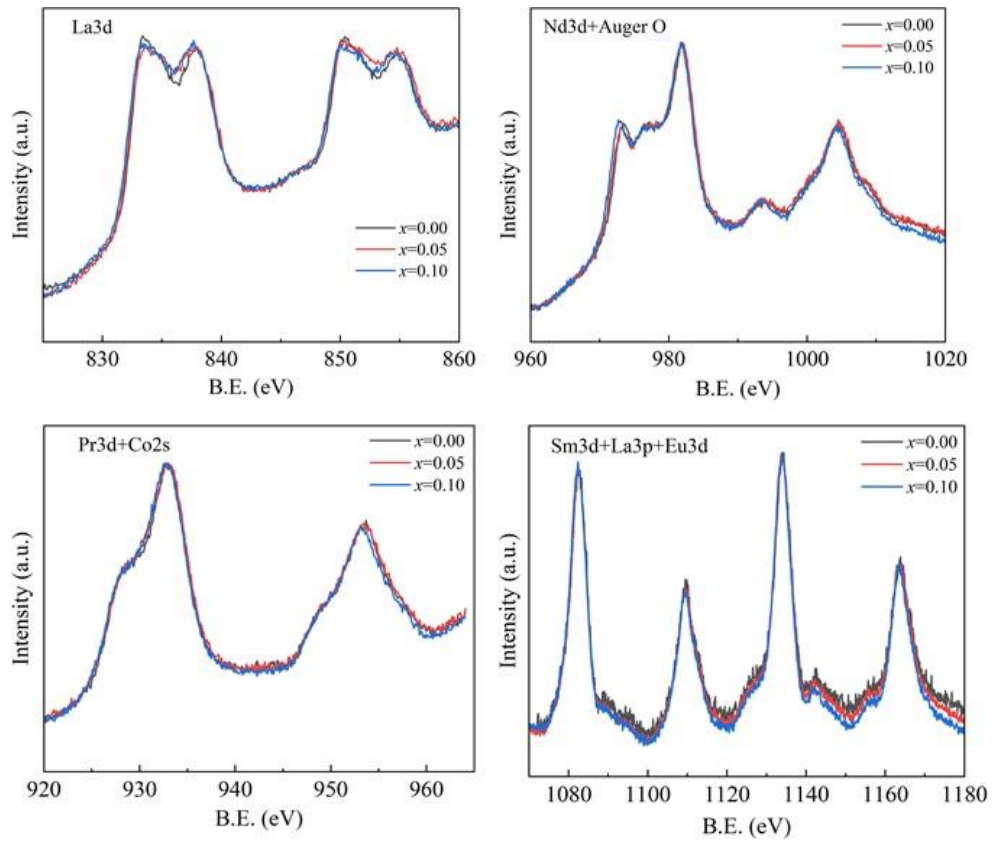

Fig.S5: Core-level spectrum for the rare-earth elements in  $(\text{LaNdPrSmEu})_{1-x}\text{Sr}_x\text{CoO}_3$ .

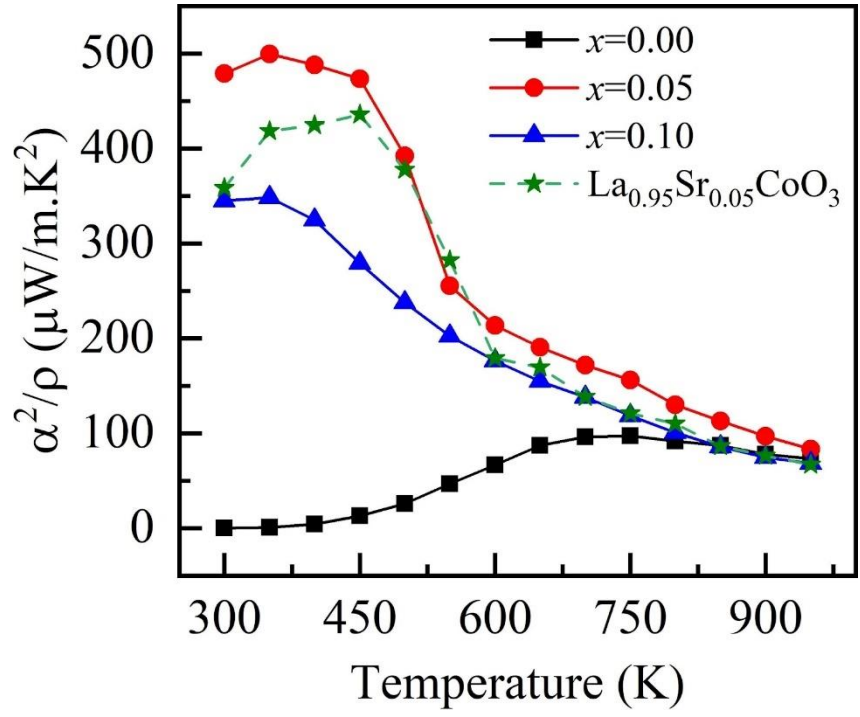

Fig.S6: Power factor ( $\alpha^2/\rho$ ) as a function of temperature for  $(\text{LaNdPrSmEu})_{1-x}\text{Sr}_x\text{CoO}_3$ . For comparison,  $\alpha^2/\rho$  for simple perovskite  $\text{La}_{0.95}\text{Sr}_{0.05}\text{CoO}_3$  is also plotted.

Table SI: Lattice parameters and goodness of fit obtained from Rietveld refinement for high-entropy  $(\text{LaNdPrSmEu})_{1-x}\text{Sr}_x\text{CoO}_3$  and simple perovskite  $\text{La}_{0.95}\text{Sr}_{0.05}\text{CoO}_3$ .

| Sample                                         | Space group | a (Å)  | b (Å)  | c (Å)   | $\chi^2$ |
|------------------------------------------------|-------------|--------|--------|---------|----------|
| $x=0.00$                                       | <i>Pbnm</i> | 5.2757 | 5.2696 | 7.4452  | 1.52     |
| $x=0.05$                                       | <i>Pbnm</i> | 5.2861 | 5.2739 | 7.4752  | 1.84     |
| $x=0.10$                                       | <i>Pbnm</i> | 5.2967 | 5.2813 | 7.4839  | 1.45     |
| $\text{La}_{0.95}\text{Sr}_{0.05}\text{CoO}_3$ | <i>R-3c</i> | 5.4463 | 5.4463 | 13.1185 | 1.26     |
